# Supplementary material for: RAF: Holistic Compilation for Deep Learning Model Training
Source: arXiv:2303.04759 source file (2023-03-08)
Supplement: Supplementary file 1 [file Appendix.tex]

\section{Appendix}
\label{sec:appendix}
\begin{table}
 \label{tab:pass}
 \caption{Passes and their IR format}
    \centering
    \begin{tabular}{|l|l|}
    \hline
        Pass Name & IR Format \\ \hline
        LiftBranchBody & ANF \\ \hline
        FlattenClosure & ANF \\ \hline
        Autodiff & ANF \\ \hline
        InlineBackward & ANF \\ \hline
         &  \\ \hline
        ToGraphNormalForm & Any → GNF \\ \hline
        ToBasicBlockNormalForm & GNF → BBNF \\ \hline
         &  \\ \hline
        AutoDataParallel & BBNF \\ \hline
        DeadCodeElimination & BBNF \\ \hline
        FuseOps & BBNF \\ \hline
        GradInputSelect & BBNF \\ \hline
        AutoCast & BBNF \\ \hline
        FoldConstant & BBNF \\ \hline
        PartitionGraph & BBNF \\ \hline
        AnnotateTarget & BBNF \\ \hline
        MergeCompilerRegions & BBNF \\ \hline
        CanonicalizeOps & BBNF \\ \hline
         &  \\ \hline
        ToANormalForm & Any → ANF \\ \hline
        ManifestAlloc & ANF \\ \hline
        InplaceUpdate & ANF \\ \hline
        DeviceAnalysis & ANF \\ \hline
        Lower to VM & ANF \\ \hline
         &  \\ \hline
        InferType & Any \\ \hline
        Substitute & Any \\ \hline
        SimplifyExpr & Any \\ \hline
    \end{tabular}
\end{table}
